# Supplementary material for: Semantically-Prompted Language Models Improve Visual Descriptions
Source: arXiv:2306.06077 source file (2024-11-22)
Supplement: Supplementary file 1 [file appendix.tex]

\end{table*}
